# Supplementary material for: ARC: Fair Relative Advantage Comparison in Open-Ended Real-World Interaction
Source: arXiv:2608.13622 source file (2026-08-13)
Supplement: Supplementary file 1 [file appendix.tex]

\section{Reproducibility Details}

Use the appendix for reader-facing methodological detail: prompts or policies
when scientifically necessary, full benchmark definitions, hyperparameters,
additional controls, and error taxonomies. Keep internal paths, run IDs, and
project-management notes in the artifact documentation rather than the paper.

\section{Additional Results}

Place supporting analyses here when they help audit the main claim but are not
required to understand the primary evidence.
